# Supplementary material for: Influence of interface and microstructure on magnetization of epitaxial Fe4N thin film
Source: arXiv:1906.01238 source file (2019-06-04)
Supplement: Supplementary file 1 [file Supplementary_Documents_final.pdf]

# Supplementary material for "Influence of interface and microstructure on magnetization of epitaxial $Fe_4N$ thin film"

Nidhi Pandey[1], S. Pütter[2], S. M. Amir[2], V. R. Reddy[1], D. M. Phase[1], J. Stahn[3], Ajay Gupta[4] and Mukul Gupta[1*]
[1] *UGC-DAE Consortium for Scientific Research, University Campus, Khandwa Road, Indore 452 001, India*
[2] *Jülich Centre for Neutron Science (JCNS) at Heinz Mair-Leibnitz Zentrum (MLZ), Forschungszentrum Jülich GmbH, Lichtenbergstr. 1, 85748 Garching, Germany*
[3] *Laboratory for Neutron Scattering and Imaging, Paul Scherrer Institut, CH-5232 Villigen PSI, Switzerland*
[4] *Amity Center for Spintronic Materials, Amity University, Sector 125, Noida 201 303, India and*
[*] *Corresponding author email: mgupta@csr.res.in*
(Dated: June 3, 2019)

### A. Morphology and Microstructure

Surface morphology of samples A, B and C grown using dcMS, HiPIMS and MBE, respectively was examined using atomic force microscopy (AFM) measurements in non-contact mode. Fig. 1 (left panel) shows the 2D AFM images of samples A, B and C. As can be seen there surface morphology differs in them. Sample B apparently exhibits a considerably denser microstructure compared to other samples A and C. In addition, grain size distribution is also like mono-dispersed in this sample. The rms roughness calculated using AFM images comes out to be about 8.1, 0.88, 2.3 nm, respectively for samples A, B and C in agreement with our XRR results.

Height histograms were extracted from AFM images using WSXM software[1] and shown in the fig. 1 (left panel) for samples A, B and C. A narrow and symmetric height distribution can be seen for sample B with skewness $\approx 0.26$ and kurtosis $\approx 3.63$ while skewness(kurtosis) of height histogram profiles for sample A and C are about 1.69(7.31) and 0.53(3.59), respectively. These results further indicate the surface morphology of sample B is superior than A or C. Utilizing AFM images, the growth modes have been explored. It is known that the interface width $\xi$ (standard deviation of the surface height) from the scaling theory can be expressed as:[2]

$$\xi(t)^2 = L^{2\alpha} \tag{1}$$

where $L$ is the length scale over which the roughness is measured, $\alpha$ is the static scaling exponents. The static scaling exponents ($\alpha$) can be used to examine the thermodynamical growing models. For Frank-van der Merwe (FM; layer by layer) growth, the surface remains flat as it grows and the value of $\alpha = 0$. Whereas, for other two models, Stranski-Krastanov (SK) and Volmer-Weber (VW) growth (island plus layer) $0.5 < \alpha < 0.6$.[2] In the present case, we find that $\alpha$ is nearly zero ($\approx 0.2$) for sample B but quite large (about 0.5 in sample A and 0.6 in C) in others. Height histogram results and the static scaling exponent $\alpha$ clearly confirm the Frank-van der Merwe type growth (layer by layer) in sample B while Stranski-Krastanov type growth (island plus layer) in samples A and C.

Here, the occurrence of different growth morphology in all samples can be understood in terms of the kinetics of adatoms during deposition. It has been previously demonstrated that by controlling and manipulating the adatom mobility during growth, one can achieve the layer by layer type growth (FM mode). This can happen when the adatom mobility is sufficiently high during the nucleation process but reduces rapidly thereafter.[3,4] Such variation in the adatom mobility can be achieved in the HiPIMS process. A high power impulse lasting about 150 $\mu$s forces adatoms to descend at the island edge while during pulse-off period (13 ms), adatoms form the rest of monolayer during the relaxation process. This mechanism may results in a layer by layer (FM) type growth in HiPIMS process also observed in other system like TiN.[5–7] On the other hand, due to continuous sputtering in dcMS, film grows in island plus layer type (SK) mode.

### B. Site-specific magnetization

In order to measure site-specific magnetization in our epitaxial samples, we deposited a 30 nm $^{57}Fe_4N$ film and did conversion electron Mössbauer spectroscopy (CEMS) measurement. Such $^{57}Fe$ enriched sample could only be prepared using dcMS due to experimental constraints (e.g. for HiPIMS a large $\phi$3-inch target of $^{57}Fe$ was required). Still, the site specific magnetization measurements provide a vital information and can be compared with the available literature.[8] It is known that in $Fe_4N$ two inequivalent Fe sites are available as shown in fig. 2. Here Fe (I) are corner sites and Fe (II) are face center sites. Both these sites possess different magnetization behavior.[8] Such occurrence of different Fe sites makes the CEMS spectra rather complicated as shown in fig. 2. Apart from these two sites, the easy axis of magnetization in $Fe_4N$ is parallel to the (100) direction, and further splits the subspectrum of Fe (II) site into an additional subspectrum with an intensity ratio of 2:1 (namely Fe (II)A and Fe (II)B shown in fig. 2).[8] In addition, since Fe (I) atoms posses cubic symmetry, the quadrupole splitting (QS) is zero. On the other hand, Fe (II) have an axial symmetry and therefore a strong hybridization with N results in a non-zero QS. The CESM spectrum was de-

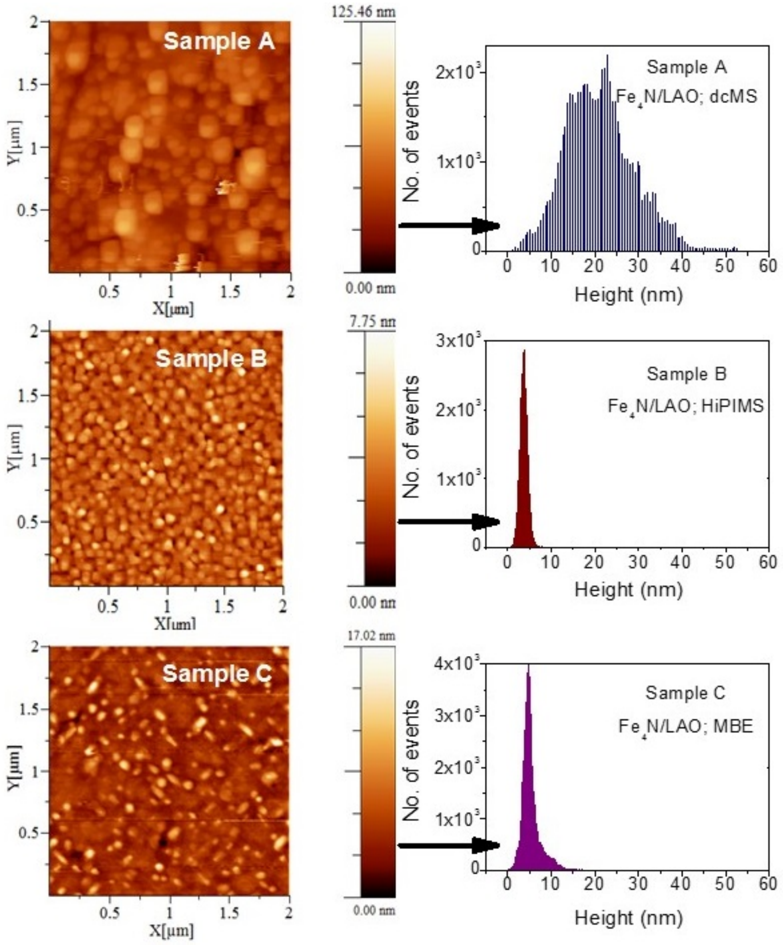


FIG. 1. Left: $2{\times}2\mu m^2$ 2D AFM images of samples A, B and C. Right: Height histogram of the corresponding AFM images shown by arrow.

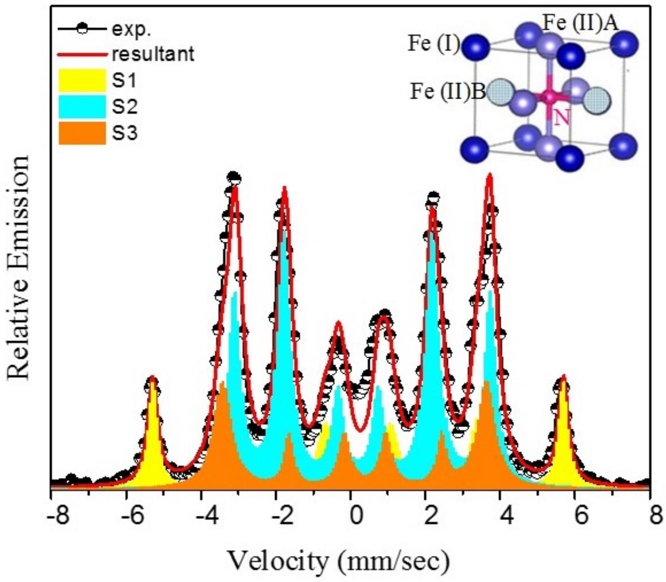


FIG. 2. Fitted CEMS spectra taken at 300 K of a $Fe_4N$ film of thickness about 30 nm grown by dcMS. A schematic representation of $Fe_4N$ structure is shown defining the different Fe sites.

TABLE I. CEMS fit parameters for $Fe_4N$ film grown using dcMS, isomer shift(IS), hyperfine field ($\mathbf{B}_{hf}$), quadrupole splitting (QS), relative area (R.A.).

| Component | IS (mm/sec) | $\mathbf{B}_{hf}$ (T) | QS (mm/sec) | R.A. % | Theoretical[10,11] $\mathbf{B}_{hf}$(T) |
|---|---|---|---|---|---|
| Fe (I) | 0.20 | 34 | 0 | 25 | 37 |
| Fe (II)A | 0.25 | 21.7 | 0.07 | 50 | 23.4 |
| Fe (II)B | 0.26 | 21.5 | -0.14 | 25 | 23.4 |

convoluted using NORMOS programme.[9] It was found that the hyperfine field ($\mathbf{B}_{hf}$) for Fe (I) site was about 34 T and for Fe (II) site it was about 21.7 T. Fitted parameters are given in Tab. I. Although the fit parameters are quite well matched with the previously reported values[8] but the values of the hyperfine fields ($\mathbf{B}_{hf}$) are smaller than the theoretical values given in Tab. I. The discrepancy between the theoretical[10,11] and experimentally values of $\mathbf{B}_{hf}$ values has been discussed in the main manuscript.

## REFERENCES


1. I. Horcas, R. Fernández, J. Gomez-Rodriguez, J. Colchero, J. Gómez-Herrero, and A. Baro, Review of Scientific Instruments **78**, 013705 (2007).
2. W. M. Tong, R. S. Williams, A. Yanase, Y. Segawa, and M. S. Anderson, Physical Review Letters **72**, 3374 (1994).
3. Z. Zhenyu *et al.*, *Morphological organization in epitaxial growth and removal*, Vol. 14 (World Scientific, 1999).
4. G. Rosenfeld, B. Poelsema, and G. Comsa, Journal of Crystal Growth **151**, 230 (1995).
5. S. Shayestehaminzadeh, E. B. Thorsteinsson, D. Primetzhofer, F. Magnus, and S. Olafsson, Journal of Physics D: Applied Physics **49**, 455301 (2016).
6. Q. Luo, S. Yang, and K. Cooke, Surface and Coatings Technology **236**, 13 (2013).
7. G. Kamath, A. Ehiasarian, and P. E. Hovsepian, IEEE Transactions on Plasma Science **38**, 3062 (2010).
8. J. L. Costa-Krämer, D. Borsa, J. M. García-Martín, M. S. Martín-González, D. Boerma, and F. Briones, Physical Review B **69**, 144402 (2004).
9. R. Brand, Wissenschaftlich Elektronik GmbH, Starnberg (1995).
10. R. Coehoorn, G. Daalderop, and H. Jansen, Physical Review B **48**, 3830 (1993).
11. P. Mohn and S. Matar, Journal of Magnetism and Magnetic Materials **191**, 234 (1999).
